# Supplementary material for: Sequential convergence of AdaGrad algorithm for smooth convex optimization
Source: arXiv:2011.12341 source file (2021-04-13)
Supplement: Supplementary file 1 [file appendixA.tex]

% \section{Remaining proofs and Lemmas}
% The following two proofs are simplification of the arguments in \cite{combettes2013variable}, we provide these details for completeness.
% \label{AppendixA}
% \subsection{Proof of Proposition \ref{prop:quasifejerproperties}}\label{proof:quasifejerproperties}
% We need the next lemma for the proof.
% \begin{lem}[\cite{polyak1987introduction}, Lemma 2.2.2]\label{lem:extraproof} Let $\left(\alpha_{k}\right)_{k \in \mathbb{N}}$ be a nonnegative sequence, let $\left(\eta_{k}\right)_{k \in \mathbb{N}} \in \ell_{+}^1$ and let $\left(\varepsilon_{k}\right)_{k \in \mathbb{N}} \in \ell_{+}^1$ such that,  $\forall k \in \mathbb{N}$, $\alpha_{k+1} \leqslant\left(1+\eta_{k}\right) \alpha_{k}+\varepsilon_{k}$. Then $\left(\alpha_{k}\right)_{k \in \mathbb{N}}$ converges.
% \end{lem}
% \begin{proof}[Proof of the proposition]\textbf{ }

% % Let $y \in \RR^n$. By induction, we get from \eqref{eq:variablemetrivfejer}, for $k \in \NN$,
% %     \begin{align*}
% %         \|u_{k+1} - y\|^2 &\leq \|u_0 - y\|^2 + \sum_{\ell=0}^{k}\varepsilon_\ell \\
% %             &\leq \|u_0 - y\|^2 + \sum_{\ell=0}^{\infty}\varepsilon_\ell\\
% %             &\leq \infty.
% %     \end{align*}
% %     Therefore $\left(u_{k}\right)_{k \in \NN}$ is bounded.
% \begin{enumerate}[(i)]
%     \item As an application of Lemma \ref{lem:extraproof} to \eqref{eq:variablemetrivfejer}, with $\alpha_k = \|u_k - u\|_{w_k}$, we have that $(\|u_k - u\|^2_{W_k})_{k \in \NN}$ converges and hence $(\|u_k - u\|_{W_k})_{k \in \NN}$. 
%     %Let's say it converges to $\lambda$. $\left(\|u_k - u\|_{W_k}\right)_{k \in \NN}$ is bounded since $x \mapsto x^2$ tends to $\infty$ when $x \rightarrow \infty$. Let's consider two subsequences $\left(\|u_{m_k} - u\|_{W_k}\right)_{m_k \in \NN}$ and $\left(\|u_{l_k} - u\|_{W_k}\right)_{l_k \in \NN}$ such that $\|u_{m_k} - u\|_{W_{m_k}} \rightarrow m_0$ and $\|u_{l_k} - u\|_{W_{l_k}} \rightarrow l_0$. We suppose that $m_0 \neq l_0$, say $m_0 < l_0$. Fix $\varepsilon \in \left( 0,(l_0-m_0) / 2\right)$. For $k$ big enough, $\|u_{m_k} - u\|_{W_{m_k}} \leq m_0 + \varepsilon < l_0 - \varepsilon \leq \|u_{l_k} - u\|_{W_{l_k}}$. It follows that $\|u_{m_k} - u\|^2_{W_{m_k}} \leq (m_0 + \varepsilon)^2 < (l_0 - \varepsilon)^2 \leq \|u_{l_k} - u\|^2_{W_{l_k}}$. Taking the limit as $k \rightarrow \infty$ gives $\lambda \leq (m_0 + \varepsilon)^2 < (l_0 - \varepsilon)^2 \leq \lambda$. That is impossible. So $m_0 = l_0$ and $(\|u_k - u\|_{W_k})_{k \in \NN}$ converges.
%     \item Let $u \in C$. By assumption, $W_k \succeq \alpha I_n, \forall k \in \NN$, for some $\alpha > 0$. So, $\forall k \in \NN$
%     \begin{align*}
%         \left\|u_{k}-u\right\|^{2} \leqslant \frac{1}{\alpha} \left\langle u_{k}-u, W_{k} \left(u_{k}-u\right) \right\rangle = \frac{\left\|u_{k}-u\right\|_{W_{k}}^{2}}{\alpha}.
%     \end{align*}
%     Thanks to the previous point $(\|u_k - u\|_{W_k})_{k \in \NN}$ is bounded, then so is $(u_k)_{k \in \NN}$.
% \end{enumerate}
% \end{proof}
% %########################################################################################
% %######################################################################################
% \subsection{Proof of Theorem \ref{thm:cnvgevarmet}}\label{proof:cvgcequasifejer}
% % \begin{lem}[\cite{bauschke2011convex}, Lemma 2.41 (ii) and (iii)]\label{lem:intermediate2}
% % Let $\left(x_{\mathrm{k}}\right)_{\mathrm{k} \in \mathrm{N}}$ and $\left(u_{k}\right)_{k \in \mathrm{N}}$ be sequences in $\mathcal{H},$ and let $x$ and $u$ be points in $\mathcal{H}$. The following hold:
% % \begin{enumerate}[(i)]
% %     \item Suppose that $\mathcal{H}$ is finite-dimensional. Then $x_{k} \rightharpoonup x \Leftrightarrow x_{k} \rightarrow x$.
% %     \item Suppose that $x_{k} \rightharpoonup x$ and $u_{k} \rightarrow u$. Then $\left\langle x_{k}, u_{k}\right\rangle \rightarrow\langle x, u\rangle$.
% % \end{enumerate}
% % \end{lem}
% \begin{proof}[Proof of the theorem]
% Let $\mathfrak{W}$ be the set of all accumulation points of $(x_k)_{k \in \NN}$. First, suppose that $x_k \rightarrow \bar{x} \in C$, as $k \to \infty$, then obviously, $\mathfrak{W} = \{\bar{x}\} \subset C$.

% Conversely suppose that $\mathfrak{W} \subset C$. $\mathfrak{W}$ is not empty since by the Proposition \ref{prop:quasifejerproperties}, $\left(x_{k}\right)_{k \in \NN}$ is bounded. Fix $x$ and $x^{\prime}$ in $\mathfrak{W}$ arbitrary. Say that $x_{m_{k}} \rightarrow x$ and $x_{l_{k}} \rightarrow x^{\prime}$ along two subsequences. From Proposition \ref{prop:quasifejerproperties} \eqref{prop:quasifejerproperties1}, we know that $\left(\left\|x_{k}-x\right\|_{W_{k}}\right)_{k \in \mathrm{N}}$ and $\left(\left\|x_{k}-x'\right\| W_{k}\right)_{k \in \mathrm{N}}$ converge since both $x$ and $x'$ are in $C$. Also for any $d \in \RR^n$, $\|d\|_{W_{k}}^{2}=\left(W_{k} d , d\right) \rightarrow\left\langle Wd, d\right\rangle$ as $k \to \infty$. Since, for all $k \in \NN$
% \begin{align*}
%     \left\langle W_{k} x_{k}, x-x^{\prime}\right\rangle = \frac{1}{2}\left(\left\|x_{k} - x^{\prime} \right\|_{W_{k}}^{2} - \left\|x_{k}-x\right\|_{W_{k}}^{2}+\|x\|_{W_{k}}^{2}-\|x^{\prime}\|_{W_{k}}^{2}\right),
% \end{align*}
% the sequence $\left(\left\langle W_{k} x_{k}, x-x^{\prime}\right\rangle\right)_{k \in \mathbb{N}}$ converges, let's say to $\lambda \in \mathbb{R},$ this means that
% \begin{align}
%     \left\langle x_{k}, W_{k}(x-x^{\prime})\right\rangle \underset{k\to \infty}{\rightarrow} \lambda \in \mathbb{R}.
%     \label{eq:intermediate}
% \end{align}
% Since, as $k \to \infty$, $x_{m_{k}} \rightarrow x$ and $W_{m_{k}}(x-x^{\prime}) \rightarrow W(x-x^{\prime}),$ it follows from \eqref{eq:intermediate} that $\langle x, W(x-x^{\prime})\rangle = \lambda$. The same way we show that $\langle x^{\prime}, W(x-y)\rangle=\lambda$.
% So
% \begin{align*}
%     0&=\langle x, W(x-x^{\prime})\rangle-\langle x^{\prime}, W(x-x^{\prime})\rangle=\langle x-x^{\prime}, W(x-x^{\prime})\rangle \\
%     &\geqslant \alpha\|x-x^{\prime}\|^{2},
% \end{align*}
% and hence we obtain $x=x^{\prime}$. Since $x$ and $x'$ were arbitrary accumulation points, the set of accumumation points is reduced to a singleton, that is $x_{k} \rightarrow x \in C$ as $k \to \infty$.
% \end{proof}

%%%%%%%%%%%%%%%%%%%%%%%%%%%%%%%%%%%%%%%%%%%%%%%%%%%%%%%%%%%%%%%%%%%%%%%%%%%%%%%%%%%%%%%%%%%%%%%%%%%%%%%%%%%%%%%%%%%%%%%%%%%%%%%%%%%%%%%%%%%%%%%%%%%%%%%%%%%%%%%%%%%%%%%%%%%%%%%%%%%%%%%%%%%%%%%%%%%%%%%%%%%%%%%%%%%%%%%%%%%%%%%%%%%%%%%

% We need the following results.
% \begin{prop}\label{prop:previouscvgcequasifejer}
% Let $\left(u_{k}\right)_{k \in \NN}$ be a quasi-Fejér sequence relative to a nonempty, convex and closed set $C$ in $\RR^n$. Then
% \begin{enumerate} [(i)]
%     \item \label{ass:previouscvgcequasifejer1} For every $x \in C$, $\left(\left\|u_{k}-x\right\|\right)_{k \in \NN}$ converges.
%     \item \label{ass:previouscvgcequasifejer2} $\forall x, x^{\prime} \in \mathfrak{W}, \exists \alpha \in \mathbb{R}, \text{ such that } C \subset\left\{y \in \RR^n \mid\left\langle y , x-x^{\prime}\right\rangle=\alpha\right\},$
% \end{enumerate}
% where $\mathfrak{W}$ is the set of the accumulation points of $\left(u_{k}\right)_{k \in \NN}$.
% \end{prop}
% \begin{proof}\textbf{ }

% \begin{enumerate}[(i)]
%     \item Let $x \in C$. Thanks to the Proposition \ref{prop:quasifejerproperties}, it is clear that $\left(\left\|u_{k}-x\right\|\right)_{k \in \NN}$ is bounded; hence it has an accumulation point. Let $\liminf{\left(\left\|u_{k}-x\right\|\right)} = \alpha$. There exists a subsequence $\left(\left\|u_{\ell_{k}}-x\right\|\right)_{\ell_{k} \in \NN}$ of $\left(\left\|u_{k}-x\right\|\right)_{k \in \NN}$ that converges to $\alpha$. 
%     Let's take $\delta > 0$. Thus there is $k_0 \in \NN$ such that
%     \begin{align*}
%         \|u_{\ell_{k_0}}-x\| - \alpha < \frac{\delta}{2} \text{ and } \sum_{m \geq \ell_{k_0}}^{\infty} \varepsilon_m < \frac{\delta}{2}.
%     \end{align*}
%     The last inequality is due to the fact that $\sum_{m = 0}^{\infty} \varepsilon_m < \infty$. But due to the equation \eqref{eq:variablemetrivfejer} and by induction, we obtain for all $k \geq \ell_{k_0}$
%     \begin{align*}
%          \|u_{k+1}-x\| &\leq \|u_{\ell_{k_0}}-x\| + \sum_{m \geq \ell_{k_0}}^{k} \varepsilon_m \\
%             &\leq \|u_{\ell_{k_0}}-x\| + \sum_{m \geq \ell_{k_0}}^{\infty} \varepsilon_m\\
%             &< \frac{\delta}{2} + \alpha + \frac{\delta}{2} \\
%             &= \liminf{\left(\left\|u_{k}-x\right\|\right)} + \delta
%     \end{align*}
%     Therefore $\limsup{\left(\left\|u_{k}-x\right\|\right)} \leq \liminf{\left(\left\|u_{k}-x\right\|\right)} + \delta$. Making $\delta$ tends to $0$, we have $\limsup{\left(\left\|u_{k}-x\right\|\right)} = \liminf{\left(\left\|u_{k}-x\right\|\right)}$. Hence $\left(\left\|u_{k}-x\right\|\right)_{k \in \NN}$ converges.
%     \item Let $y \in C. $Then let's consider two points $x$ and $x^{\prime}$ in $\mathfrak{W}$ and two subsequences that converge to those points, $u_{m_{k}} \rightarrow x$ and $u_{\ell_{k}} \rightarrow x^{\prime}.$ We know that, $\forall k \in \mathbb{N},$ $$\left\|u_{k}-y\right\|^{2}-\|y\|^{2}=\left\|u_{k}\right\|^{2}-2\left\langle y, u_{k}\right\rangle.$$
% From Proposition \ref{prop:previouscvgcequasifejer} \eqref{ass:previouscvgcequasifejer1}, we obtain that $\gamma=\lim \left\|u_{k}-y\right\|^{2}-\|y\|^{2}$ exists and is finite. Thus, by continuity of the inner product,
% $$
% \gamma=\lim \left\|u_{m_{k}}\right\|^{2}-2\langle y, x\rangle=\lim \left\|u_{\ell_{k}}\right\|^{2}-2\left\langle y, x^{\prime}\right\rangle
% $$
% So
% \begin{align*}
%     \langle y, x - x^{\prime}\rangle = \left(\lim \left\|u_{m_{k}}\right\|^{2}-\lim \left\|u_{\ell_{k}}\right\|^{2}\right) / 2.
% \end{align*}
% Therefore by setting $\alpha=\left(\lim \left\|u_{m_{k}}\right\|^{2}-\lim \left\|u_{\ell_{k}}\right\|^{2}\right) / 2$, we got the result.
% \end{enumerate}
% \end{proof}
% \begin{proof}[Proof of the theorem]
% Suppose that $u_k \rightarrow \bar{u} \in C$. Obviously, $\mathfrak{W} = \{\bar{u}\} \subset C$.

% Conversely suppose that $\mathfrak{W} \subset C$. $\mathfrak{W}$ is not empty since by the Proposition \ref{prop:quasifejerproperties}, $\left(u_{k}\right)_{k \in \NN}$ is bounded. We can take $x$ and $x^{\prime}$ in $\mathfrak{W}$. As $x, x^{\prime} \in C,$ the Proposition \ref{prop:previouscvgcequasifejer} \eqref{ass:previouscvgcequasifejer2} says that 
% \begin{align*}
%     \left\langle x , x-x^{\prime}\right\rangle = \left\langle x^{\prime}, x-x^{\prime}\right\rangle &\Longleftrightarrow \|x - x^{\prime}\| = 0 \\
%     &\Longrightarrow x = x^{\prime}.
% \end{align*}
% That means $\mathfrak{W}$ is a singleton, hence $\left(u_{k}\right)_{k \in \NN}$ converges.

% \end{proof}


% \subsection{Technical lemmas}
% \label{AppendixB}
% \begin{lem}\label{lem:quadratic}
% Let $a,b \geq 0$. If for $Z \geq 0$, $\displaystyle \frac{Z}{\sqrt{Z+a}} \leq b$, then $\displaystyle Z \leq b^2 + b\sqrt{a}$.
% \end{lem}
% \begin{proof}
% We have 
% \begin{align*}%\label{eq:quadratic}
%     Z^2 - b^2Z - b^2a \leq 0.
% \end{align*}
% For the equation of second order, $\Delta = b^4 + 4b^2a \geq 0$. We have two distinct real roots and the leading coefficient is positive, so for $Z$ to satisfy the above inequality, we should have
% \begin{align*}
%     Z &\leq \frac{b^2 + \sqrt{b^4 + 4b^2a}}{2} \\
%       &\leq \frac{b^2 + \sqrt{b^4} + \sqrt{4b^2a}}{2} \\
%       &= b^2 + b\sqrt{a}.
% \end{align*}
% \end{proof}

%%%%%%%%%%%%%%%%%%%%%%%%%%%%%%%%%%%%%%%%%%%%%%%%%%%%%%%%%%%%%%%%%%%%%%%%%%%%%%%%%%%%%%%%%%%%%%%%%%%%%%%%%%%%%%%%%%%%%%%%%%%%%%%%%%%%%%%%%%%%%%%%%%%%%%%%%%


% \section{On the importance of full domain assumption}
% \label{AppendixC}
% Do Algorithm \eqref{algo:adagradSimple} or \eqref{algo:adagradSimplecoord} converge when the global Lipschcity assumption is relaxed to local Lipschicity. We argue that full domain assumption would be essential for such a result. This section provides a counter example in dimension 1 of a convex function on $(-1/2,1/2)$ with locally Lipschitz derivative and an Adagrad sequence which is divergent. Note that in dimension 1, both algorithms are the same.

% \begin{lem}
%     \label{lem:interpolationDim1}
%     Let $(x_k)_{k\in \NN}$ and $(z_k)_{k\in \NN}$ be two real sequence such that
%     \begin{itemize}
%         \item $x_1 < x_0$ and $z_1 \leq z_0$.
%         \item $(x_{2k})_{k\in \NN}$ is strictly increasing and $(z_{2k})_{k\in \NN}$ is non decreasing.
%         \item $(x_{2k+1})_{k\in \NN}$ is strictly decreasing and $(z_{2k+1})_{k\in \NN}$ is non increasing.
%     \end{itemize}
%     Then there exists a differentiable convex function $f \colon (\inf_{k \in \NN} x_k, \sup_{k \in \NN} x_k) \to \RR$ with locally Lipschitz gradient such that for all $k \in \NN$, $f'(x_k) = z_k$.
% \end{lem}   
% \begin{proof}
%     For each $k > 1$, define
%     \begin{itemize}
%         \item $g_k \colon [x_0, x_{2k}] \to \RR$ to be the affine interpolant such that $g_k(x_{2i}) = z_{2i}$ for all $i = 0,\ldots k$.
%         \item $h_k \colon [x_{2k+1},x_0] \to \RR$ to be the affine interpolant such that $h_k(x_{2i+1}) = z_{2i+1}$ for all $i = 0,\ldots k$ and $h_k(x_0) = z_0$.
%         \item $f_k \colon [x_{2k+1},x_{2k}] \to \RR$ be such that $f_k(x) = \int_{x_0}^x g_k(t) dt$ for $x \geq 0$ and $f_k(x) = \int_{x_0}^x h_k(t) dt$ for $x < 0$.
%     \end{itemize}
%     $f_k$ is continuously differentiable on $(x_{2k+1},x_{2k})$ and we have for all $x \in (x_{2k+1},x_{2k})$ that $f_k'(x) = g_k(x)$ if $x \geq 0$ and $f'_k(x) = h_k(x)$ if $x < 0$. Its derivative is non decreasing and hence $f_k$ is convex and its derivative is locally Lipschitz because it is piecewise affine.
    
%     For $k' \geq k$, the function $f_{k'}$ defined on $[x_{2k'+1},x_{2k'}]$ agrees with $f_k$ on $[x_{2k+1},x_{2k}] \subset [x_{2k'+1},x_{2k'}]$. The desired function $f$ is defined for any $x \in (\inf_{k \in \NN} x_k, \sup_{k \in \NN} x_k)$ to be the equal to $f_k(x)$ for any $k$ such that $x \in (x_{2k+1},x_{2k})$, such a $k$ must exist by properties of infimum and suppremum. This is the desired function $f$.
% \end{proof}
% We need a last technical lemma.
% \begin{lem}
%     Let $0<b<1$, $\delta>0$ and $c>0$. Setting
%     \begin{align*}
%         a = \pm \frac{b}{\sqrt{1 - b^2}} \sqrt{\delta + c},
%     \end{align*}
%     we have
%     \begin{align}
%         \frac{a^2}{\delta + c + a^2} = b^2.
%     \end{align}
%     \label{lem:technicalCounterEx}
% \end{lem}
% \begin{proof}
%     We have
%     \begin{align*}
%         a^2 &= \frac{b^2}{1 - b^2} (\delta + c)\\
%         &=\frac{b^2}{1 - b^2} (\delta + c + a^2) - a^2 \frac{b^2}{1 - b^2}.
%     \end{align*}
%     We deduce that
%         \begin{align*}
%         \frac{a^2}{1 - b^2} &=\frac{b^2}{1 - b^2} (\delta + c + a^2),
%     \end{align*}
%     and the desired result follows
% \end{proof}

% Consider the following sequence
% \begin{itemize}
%     \item $x_{2k} = \frac{1}{2} - \frac{1}{2^{k+1}}$, for all $k \in \NN$.
%     \item $x_{2k+1} = \frac{-1}{2} + \frac{1}{2^{k+2}}$, for all $k \in \NN$.
% \end{itemize}
% This sequence complies with the hypotheses of Lemma \ref{lem:interpolationDim1}.  Furthermore, $|x_k - x_{k+1}|$ is an increasing sequence, strictly smaller than $1$. Fix $\delta = 15$ and $z_0 = 1$. This ensures that $x_0 - z_0 / \sqrt{\delta + z_0^2} = x_1$. This relation will be preserved by recursion, setting for all $k \in \NN$
% \begin{itemize}
%     \item $z_{2k+1} = - \frac{|x_{2k+2} - x_{2k+1}|}{\sqrt{1 - |x_{2k+2} - x_{2k+1}|^2}}  \sqrt{\delta + \sum_{i=0}^{2k} z_i^2}$.
%     \item $z_{2k+2} =   \frac{|x_{2k+3} - x_{2k+2}|}{\sqrt{1 - |x_{2k+3} - x_{2k+2}|^2}}  \sqrt{\delta + \sum_{i=0}^{2k+1} z_i^2}$.
% \end{itemize}
% We have for all $k \in \NN$,
% \begin{align*}
%     \frac{|z_{2k+1}|}{\sqrt{\delta + \sum_{i=0}^{2k+1}z_i^2}} = |x_{2k+2} - x_{2k+1}|,
% \end{align*}
% by using Lemma \ref{lem:technicalCounterEx} with $a = |z_{2k+1}|$, $b =  |x_{2k+2} - x_{2k+1}|$, $c =\sum_{i=0}^{2k} z_i^2$ and the chosen value of $\delta$. Similarly, for all $k \in \NN$, by using Lemma \ref{lem:technicalCounterEx} with $a = |z_{2k+2}|$, $b =  |x_{2k+3} - x_{2k+2}|$, $c =\sum_{i=0}^{2k+1} z_i^2$, 
% \begin{align*}
%     \frac{|z_{2k+2}|}{\sqrt{\delta + \sum_{i=0}^{2k+2} z_i^2}} = |x_{2k+3} - x_{2k+2}|,
% \end{align*}
% In summary, we have for all $k \in \NN$,
% \begin{align}
%     \label{eq:tempInterpol1}
%     \frac{|z_{k}|}{\sqrt{\delta + \sum_{i=0}^{k}z_i^2}} = |x_{k+1} - x_{k}|.
% \end{align}
% Carefully studying the signs of each sequence, we have for all $k \in \NN$
% \begin{align*}
%     \frac{z_{2k}}{\sqrt{\delta + \sum_{i=0}^{2k}} z_i^2} = x_{2k} - x_{2k+1} & \geq 0\\
%     \frac{z_{2k+1}}{\sqrt{\delta +\sum_{i=0}^{2k+1}} z_i^2} = x_{2k+1} - x_{2k+2} & \leq 0
% \end{align*}
% and finally for all $k \in \NN$
% \begin{align}
%     \label{eq:tempInterpol2}
%     x_k - \frac{z_{k}}{\sqrt{\delta + \sum_{i=0}^{k}} z_i^2} = x_{k+1}, 
% \end{align}
% so that the two sequences comply with recursion \eqref{eq:adagradSimple} with $z_k$ in place of derivatives. Let us check that the sequence $(z_k)_{k \in \NN}$ complies with Lemma \ref{lem:interpolationDim1}, which would conclude the proof. Given the alternating sign pattern of the sequence, it is sufficient to show that $|z_k|_{k \in \NN}$ is non decreasing. From \eqref{eq:tempInterpol1} and the fact that $|x_{k+1} - x_{k}|$ is increasing with $k$, we have for all $k \in \NN$
% \begin{align*}
%     \frac{|z_{k}|}{|z_{k+1}|} \leq \frac{\sqrt{\delta + \sum_{i=0}^{k}z_i^2}}{\sqrt{\delta + \sum_{i=0}^{k+1}z_i^2}} < 1,
% \end{align*}
% because for all $k \in \NN$, $z_{k+1}^2 > 0$. The proof is complete.
