# Supplementary material for: Sequential convergence of AdaGrad algorithm for smooth convex optimization
Source: arXiv:2011.12341 source file (2021-04-13)
Supplement: Supplementary file 2 [file appendixB.tex]

\section{Technical lemmas}

\label{AppendixB}
\begin{lem}\label{lem:quadratic}
Let $a,b \in \RR$. If for $Z \in \RR$, $\displaystyle \frac{Z}{\sqrt{Z+a}} \leq b$, then $\displaystyle Z \leq b^2 + b\sqrt{a}$.
\end{lem}
\begin{proof}
We have 
\begin{align*}%\label{eq:quadratic}
    Z^2 - b^2Z - b^2a \leq 0.
\end{align*}
For the equation of second order, $\Delta = b^4 + 4b^2a$. So for $Z$ to satisfy the above inequality, we should have
\begin{align*}
    Z &\leq \frac{b^2 + \sqrt{b^4 + 4b^2a}}{2} \\
      &\leq \frac{b^2 + \sqrt{b^4} + \sqrt{4b^2a}}{2} \\
      &= b^2 + b\sqrt{a}.
\end{align*}
\end{proof}
